# Supplementary material for: FedGen: Generalizable Federated Learning for Sequential Data
Source: arXiv:2211.01914 source file (2023-05-30)
Supplement: Supplementary file 1 [file appendix.tex]

\appendix

\section{Appendix}\label{sec:appendix}
 
 \subsection{Proof of Theorem 2}
%  \ref{thm:fedgen_convex_convergence}}\label{app:fedgen_convex_convergence}
 
 \begin{proof}
Since $F(Z, w)$ is L-smooth, we have
\begin{align}
    \begin{split}
    &F(Z^{t+1}, w^{t+1}) - F(Z^t, w^t) \\
    &\leq \langle \nabla F(Z^t, w^t), w^{t+1} - w^t \rangle + \frac{L}{2} || w^{t+1} - w^t ||^2 \\
    &\leq -\nabla F(Z^t, w^t)^\top \eta \nabla f_k(Z^t, w^t) + \frac{L}{2} || \eta \nabla f_k(Z^t, w^t) ||^2
    \end{split}
\end{align}
With Assumption 1 and B-local dissimilarity, we get
\begin{align}\label{eq:convex_convergence}
    \begin{split}
        &\mathbb{E}[F(Z^{t+1}, w^{t+1})] - F(Z^t, w^t) \\ 
        &\leq -\eta \nabla F(Z^t, w^t)^\top \mathbb{E}[\nabla f_k(Z^t, w^t)] + \frac{L\eta^2}{2} \mathbb{E}[ || \nabla f_k(Z^t, w^t) ||^2] \\
        &\leq -\eta \epsilon || \nabla F(Z^t, w^t) ||^2 + \frac{L \eta^2 B^2}{2} || \nabla F(Z^t, w^t) ||^2 \\
        &\leq -\eta(\epsilon - \frac{L \eta B^2}{2}) || \nabla F(Z^t, w^t) ||^2
    \end{split}
\end{align}

Setting $\rho = -\eta(\epsilon - \frac{L\eta B^2}{2})$ we get, 
\begin{equation}\label{eq:L_smooth_complete}
    \mathbb{E}[F(Z^{t+1}, w^{t+1})] - F(Z^t, w^t) \leq  - \rho ||\nabla F(Z^t, w^t)||^2
\end{equation}

Since $F(Z, w)$ is $\mu$-strongly convex, for some $Z'$ and $w'$, we get:
\begin{equation}\label{eq:mu_convex_first}
    F(Z', w') - F(Z^t, w^t) \geq \nabla F(Z^t, w^t)^\top (w' - w^t) + \frac{\mu}{2} || w' - w^t ||^2
\end{equation}

Since $F(Z', w')$ is quadratic in $w'$, its minimal value is obtained when $\nabla F(Z', w') = \nabla F(Z^t, w^t) + \mu (w' - w^t) = 0$. 
This occurs when $w' = w^t - \frac{\nabla F(Z^t, w^t)}{\mu}$. 
Substituting for $w'$ in Equation \ref{eq:mu_convex_first} we get,
\begin{equation}
    F(Z_*, w_*) \geq F(Z', w') \geq F(Z^t, w^t) -  \frac{|| \nabla F(Z^t, w^t) ||^2}{2\mu}
\end{equation}

\begin{equation}
    2 \mu (F(Z^t, w^t) - F(Z_*, w_*)) \leq || \nabla F(Z^t, w^t) ||^2
\end{equation}

Substituting into Equation \ref{eq:L_smooth_complete} we get, 
\begin{equation}
    \mathbb{E}[F(Z^{t+1}, w^{t+1})] - F(Z^t, w^t) \leq  - 2 \mu \rho (F(Z^t, w^t) - F(Z_*, w_*))
\end{equation}
Re-arranging and subtracting $F(Z_*, w_*)$ from both sides, 
\begin{equation}
    \mathbb{E}[F(Z^{t+1}, w^{t+1})] - F(Z_*, w_*) \leq (1 - 2 \mu \rho) (F(Z^t, w^t) - F(Z_*, w_*))
\end{equation}

\end{proof}

 \subsection{Proof of Theorem 3}
%  \ref{thm:fedgen_nonconvex_convergence}}\label{app:fedgen_nonconvex_convergence}
 
 \begin{proof}
By taking the full expectation of Equation \ref{eq:convex_convergence}, we get
\begin{equation}\label{eq:non-convex_1}
    \mathbb{E}[F(Z^{t+1}, w^{t+1})] \leq \mathbb{E}[F(Z^t, w^t)] - \rho \mathbb{E}[|| \nabla F(Z^t, w^t) ||^2]
\end{equation}
Then summing up Equation \ref{eq:non-convex_1} over global iteration T, we obtain
\begin{equation}
    \mathbb{E}[F(Z^{t+1}, w^{t+1})] \leq F(Z^0, w^0) - \sum_{t=0}^{T-1} \rho \mathbb{E}[|| \nabla F(Z^t, w^t) ||^2]
\end{equation}
From Assumption 1, we see that $F(Z^*, w^*) \leq \mathbb{E}[F(Z^{t+1}, w^{t+1})]$, using which we can write
\begin{equation}
    F(Z^*, w^*) \leq F(Z^0, w^0) - \frac{1}{T}\sum_{t=0}^{T-1} \eta \rho \mathbb{E}[|| \nabla F(Z^t, w^t) ||^2]
\end{equation}
Re-arranging,
\begin{equation}
    \frac{1}{T}\sum_{t=0}^{T-1} \rho \mathbb{E}[|| \nabla F(Z^t, w^t) ||^2] \leq F(Z^0, w^0) - F(Z^*, w^*)
\end{equation}
\end{proof}

 \subsection{Implementation Details}\label{app:implementation_details}
We simulate the federated learning setup (1 server and $N$ devices) on a commodity machine with 7 Intel\textsuperscript{\textregistered} Xeon\textsuperscript{\textregistered} E5-2690 v4 CPUs and an NVIDIA\textsuperscript{\textregistered} Tesla P100 GPU.  

We describe the implementation details of the experiments in the paper as described in Section 4.
We searched for hyper-parameters based on the values in Table \ref{tab:hyperparameter}, and chose the configurations with the best performance for each of the approaches.

\begin{table}[!h]
\centering
\resizebox{0.27\textwidth}{!} {%
    \begin{tabular}{lc} \toprule
    Hyper-parameter & Range 
    \\ 
     \midrule
     Learning rate & [$10^{-5}, 10^{-1}$] \\
     Rounds & [$11, 201$] \\
     Epochs & [$5, 150$] \\
     Regularization weight & [$10^{-6}, 10^{-2}$] \\
     Penalty & [$10, 10^4$] \\
     Scaling factor & [$10^{-2}, 10$] \\
     Proximal term (FedProx) & [$10^{-5}, 10^{-1}$] \\
     \bottomrule
    \end{tabular}%
    }
    \caption{Hyper-parameter ranges tried for all comparison approaches}
    \label{tab:hyperparameter}
\end{table}

% We consider the models to converge when the loss difference between two consecutive communication rounds $|F^{t} - F^{t-1}| < 10^{-4}$, and consider the models to diverge when we observe 
% $|F^{t} - F^{t-10}| > 1$, similar to definitions by prior work \cite{li2018federated, sahu2018convergence}.

\noindent
For both the SST-2 and AG News datasets, we used a 3-layer (50-50-2) MLP with ReLU activations, based on the average of the 50-dimensional GloVe (\texttt{glove.6B.50d}) embedding word vectors as inputs. These are pre-trained word vector embeddings that have been trained on Wikipedia articles. We achieve similar results with the 300-dimensional word vectors as well (\texttt{glove.6B.300d}). 
For SST-2, we use a learning rate of $0.001$ and set the penalty and regularizer weight for FedGen to be $10^4$ and $10^{-3}$ respectively with a scaling factor of $10$. The regularizer weight for ERM, FedAvg, Inv-FedAvg and FedProx was set to $10^{-6}$ and the proximal term was $10^{-3}$.

For AG News, we also use a learning rate of $0.001$ and set the penalty and regularizer weight for FedGen to be $1$ and $10^{-6}$ respectively with a scaling factor of $10$. The same regularizer weight was used for the other approaches and the proximal term was $10^{-3}$.

For the HAR dataset, we use an LSTM with one layer and hidden size of $100$, followed by a linear layer of size $100$ with ReLU activation. We use a batch size of $2^6$ on the clients and a learning rate of $0.01$. The regularizer weight for all approaches was set to $10^{-3}$ and FedGen's penalty was $10$ with a scaling factor of $10$. We used the same proximal term as above. 

For the Water Quality dataset, we used a 3-layer MLP (200-200-1) with ReLU activations. The learning rate was $0.07$ and the regularizer weight was $10^{-6}$. We set FedGen's penalty to $1$ with a scaling factor of $10$. 

For BPIC 2018, we use an LSTM with two layers and a hidden size of $120$ followed by a linear layer of size $120$ with ReLU activation. We use a batch size of $5\%$ on the clients. The learning rate was $0.005$ and the regularizer weight was $7e^{-6}$. We set the penalty of FedGen to $1$ and the scaling factor to $10$.
